# Supplementary material for: Accelerating core-level $GW$ calculations by combining the contour deformation approach with the analytic continuation of $W$
Source: arXiv:2305.15955 ancillary file (2023-10-20)
Supplement: Supplementary file 1 [file supplementary_information.pdf]

# Supporting Information: Accelerating core-level GW calculations by combining the contour deformation approach with the analytic continuation of W.

Ramón L. Panadés-Barrueta* and Dorothea Golze*

*Faculty of Chemistry and Food Chemistry, Technische Universität Dresden, 01062 Dresden, Germany*

E-mail: ramon_lorenzo.panades-barrueta@tu-dresden.de; dorothea.golze@tu-dresden.de

## 1 CORE65 binding energies

**Table S1:** Comparison of the CORE65 binding energies obtained with CD and CD-WAC at the $G_0W_0$@PBEh($\alpha$=0.45) level of theory and different basis sets. The MAE and MAD values of CD-WAC with respect to CD are also reported.

| | | | cc–pvTZ | | cc–pvQZ | |
|---|---|---|---|---|---|---|
| name | formula | core level | CD | CD-WAC(20, 20, 200) | CD | CD-WAC(20, 20, 200) |
| 74-82-8 | $CH_4$ | C1s | 290.20 | 290.20 | 290.40 | 290.40 |
| 74-84-0 | $C_2H_6$ | C1s | 290.18 | 290.18 | 290.39 | 290.38 |
| 74-85-1 | $C_2H_4$ | C1s | 290.35 | 290.35 | 290.54 | 290.54 |
| 74-86-2 | $C_2H_2$ | C1s | 290.80 | 290.80 | 290.89 | 290.90 |
| 630-08-0 | CO | O1s | 541.15 | 541.15 | 541.18 | 541.18 |
| 630-08-0 | CO | C1s | 295.48 | 295.48 | 295.58 | 295.58 |
| 124-38-9 | $CO_2$ | O1s | 540.22 | 540.22 | 540.28 | 540.28 |
| 124-38-9 | $CO_2$ | C1s | 297.39 | 297.39 | 297.61 | 297.61 |
| 75-73-0 | $CF_4$ | F1s | 693.65 | 693.65 | 693.61 | 693.61 |
| 75-73-0 | $CF_4$ | C1s | 301.60 | 301.60 | 301.91 | 301.91 |
| 593-53-3 | $CH_3F$ | F1s | 690.81 | 690.81 | 690.78 | 690.78 |
| 593-53-3 | $CH_3F$ | C1s | 293.00 | 293.00 | 293.27 | 293.26 |
| 75-46-7 | $CHF_3$ | F1s | 692.70 | 692.70 | 692.67 | 692.67 |
| 75-46-7 | $CHF_3$ | C1s | 298.76 | 298.76 | 299.08 | 299.08 |
| 67-56-1 | $CH_3OH$ | O1s | 537.93 | 537.93 | 537.98 | 537.98 |

**Table S1:** Continued

| name | formula | core level | CD | CD-WAC(20, 20, 200) | CD | CD-WAC(20, 20, 200) |
|---|---|---|---|---|---|---|
| 67-56-1 | $CH_3OH$ | C1s | 291.91 | 291.91 | 292.16 | 292.16 |
| 50-00-0 | $CH_2O$ | O1s | 538.15 | 538.15 | 538.21 | 538.21 |
| 50-00-0 | $CH_2O$ | C1s | 294.03 | 294.03 | 294.27 | 294.27 |
| 115-10-6 | $CH_3OCH_3$ | O1s | 537.56 | 537.56 | 537.61 | 537.61 |
| 115-10-6 | $CH_3OCH_3$ | C1s | 291.72 | 291.72 | 291.96 | 291.96 |
| 64-18-6 | HCOOH | O1s (OH) | 539.56 | 539.56 | 539.63 | 539.63 |
| 64-18-6 | HCOOH | O1s (C=O) | 537.68 | 537.68 | 537.75 | 537.75 |
| 64-18-6 | HCOOH | C1s | 295.36 | 295.36 | 295.62 | 295.63 |
| 67-64-1 | $(CH_3)_2CO$ | O1s | 536.76 | 536.76 | 536.82 | 536.82 |
| 67-64-1 | $(CH_3)_2CO$ | C1s (C=O) | 293.41 | 293.38 | 293.59 | 293.60 |
| 67-64-1 | $(CH_3)_2CO$ | C1s ($CH_3$) | 290.69 | 290.69 | 290.91 | 290.91 |
| 107-31-3 | $HCO_2CH_3$ | O1s ($OCH_3$) | 538.95 | 538.95 | 539.01 | 539.01 |
| 107-31-3 | $HCO_2CH_3$ | O1s (C=O) | 537.30 | 537.30 | 537.37 | 537.37 |
| 64-19-7 | $CH_3COOH$ | O1s (OH) | 539.05 | 539.05 | 539.12 | 539.12 |
| 64-19-7 | $CH_3COOH$ | O1s (C=O) | 537.04 | 537.04 | 537.12 | 537.12 |
| 64-19-7 | $CH_3COOH$ | C1s (COOH) | 295.03 | 295.00 | 295.26 | 295.27 |
| 64-19-7 | $CH_3COOH$ | C1s ($CH_3$) | 291.10 | 291.10 | 291.33 | 291.34 |
| 7732-18-5 | $H_2O$ | O1s | 538.55 | 538.55 | 538.60 | 538.60 |
| 10028-15-6 | $O_3$ | O1s middle | 546.73 | 546.73 | 546.79 | 546.79 |
| 10028-15-6 | $O_3$ | O1s terminal | 540.72 | 540.72 | 540.74 | 540.74 |
| 7782-44-7 | $O_2$ | O1s weaker | 543.37 | 543.37 | 543.36 | 543.36 |
| 7782-44-7 | $O_2$ | O1s stronger | 542.33 | 542.33 | 542.32 | 542.33 |
| 7727-37-9 | $N_2$ | N1s | 409.08 | 409.08 | 409.21 | 409.21 |
| 7664-41-7 | $NH_3$ | N1s | 404.73 | 404.73 | 404.91 | 404.91 |
| 74-90-8 | HCN | N1s | 405.96 | 405.96 | 406.17 | 406.10 |
| 74-90-8 | HCN | C1s | 292.80 | 292.80 | 292.94 | 292.95 |
| 75-05-8 | $CH_3CN$ | N1s | 404.85 | 404.84 | 405.00 | 405.00 |
| 75-05-8 | $CH_3CN$ | C1s ($CH_3$) | 292.22 | 292.22 | 292.45 | 292.45 |
| 75-05-8 | $CH_3CN$ | C1s (CN) | 292.19 | 292.19 | 292.35 | 292.35 |
| 56-40-6 | $C_2H_5NO_2$ | O1s (OH) | 539.12 | 539.12 | 539.20 | 539.20 |
| 56-40-6 | $C_2H_5NO_2$ | O1s (C=O) | 537.16 | 537.16 | 537.25 | 537.25 |
| 56-40-6 | $C_2H_5NO_2$ | N1s | 404.80 | 404.80 | 404.96 | 404.96 |
| 56-40-6 | $C_2H_5NO_2$ | C1s (COOH) | 294.83 | 294.83 | 295.10 | 295.10 |
| 56-40-6 | $C_2H_5NO_2$ | C1s ($CH_2$) | 291.86 | 291.86 | 292.10 | 292.11 |
| 110-86-1 | $C_5H_5N$ | N1s | 404.15 | 404.22 | 404.33 | 404.33 |
| 109-97-7 | $C_4H_4NH$ | N1s | 405.65 | 405.63 | 405.75 | 405.74 |
| 62-53-3 | $C_6H_5NH_2$ | N1s | 404.43 | 404.44 | 404.62 | 404.62 |
| 57-13-6 | $CO(NH_2)_2$ | O1s | 535.91 | 535.91 | 536.00 | 536.00 |
| 57-13-6 | $CO(NH_2)_2$ | N1s | 405.40 | 405.38 | 405.58 | 405.58 |
| 57-13-6 | $CO(NH_2)_2$ | C1s | 294.51 | 294.54 | 294.83 | 294.83 |
| 74-89-5 | $CH_3NH_2$ | N1s | 404.51 | 404.52 | 404.55 | 404.61 |
| 98-95-3 | $C_6H_5NO_2$ | O1s | 537.64 | 537.64 | 537.70 | 537.70 |
| 98-95-3 | $C_6H_5NO_2$ | N1s | 411.70 | 411.69 | 411.87 | 411.89 |
| 98-95-3 | $C_6H_5NO_2$ | C1s (C1) | 291.84 | 291.84 | 292.01 | 292.01 |
| 98-95-3 | $C_6H_5NO_2$ | C1s (C2-4) | 290.74 | 290.73 | 290.90 | 290.90 |
| 71-43-2 | $C_6H_6$ | C1s | 289.89 | 289.89 | 290.09 | 290.08 |
| 536-74-3 | $C_8H_6$ | C1s (C3) | 290.68 | 290.70 | 290.88 | 290.88 |
| 536-74-3 | $C_8H_6$ | C1s (C2) | 290.17 | 290.17 | 290.34 | 290.34 |
| 536-74-3 | $C_8H_6$ | C1s (C4-6) | 290.00 | 289.99 | 290.17 | 290.17 |
| 536-74-3 | $C_8H_6$ | C1s (C1) | 289.61 | 289.61 | 289.75 | 289.76 |

**Table S1:** Continued

| name | formula | core level | CD | CD-WAC(20, 20, 200) | CD | CD-WAC(20, 20, 200) |
|---|---|---|---|---|---|---|
| | | | | | | |
| MAE | | | | $4.408 \cdot 10^{-3}$ | | $4.314 \cdot 10^{-3}$ |
| MAD | | | | $5.000 \cdot 10^{-4}$ | | $9.500 \cdot 10^{-4}$ |

**Table S2:** Comparison of the CORE65 binding energies obtained with CD and CD-WAC at the ev$GW_0$@PBE and ev$GW$@PBE levels of theory with the cc–pvTZ basis set. The MAE and MAD values of CD-WAC with respect to CD are also reported.

| | | | ev$GW_0$@PBE | | ev$GW$@PBE | |
|---|---|---|---|---|---|---|
| name | formula | core level | CD | CD-WAC(20, 20, 200) | CD | CD-WAC(20, 20, 200) |
| 74-82-8 | $CH_4$ | C1s | 289.83 | 289.81 | 291.59 | 291.59 |
| 74-84-0 | $C_2H_6$ | C1s | 289.73 | 289.71 | 291.42 | 291.41 |
| 74-85-1 | $C_2H_4$ | C1s | 290.02 | 289.92 | 291.72 | 291.70 |
| 74-86-2 | $C_2H_2$ | C1s | 290.51 | 290.35 | 292.18 | 292.14 |
| 630-08-0 | CO | O1s | 541.27 | 541.50 | 543.56 | 543.55 |
| 630-08-0 | CO | C1s | 295.10 | 294.86 | 296.79 | 296.78 |
| 124-38-9 | $CO_2$ | O1s | 540.03 | 540.08 | 542.24 | 542.24 |
| 124-38-9 | $CO_2$ | C1s | 296.14 | 296.24 | 297.82 | 297.81 |
| 75-73-0 | $CF_4$ | F1s | 693.36 | 693.02 | 696.05 | 696.04 |
| 75-73-0 | $CF_4$ | C1s | 299.89 | 299.92 | 301.90 | 301.89 |
| 593-53-3 | $CH_3F$ | F1s | 690.98 | 690.75 | 693.34 | 693.35 |
| 593-53-3 | $CH_3F$ | C1s | 292.45 | 292.39 | 294.25 | 294.24 |
| 75-46-7 | $CHF_3$ | F1s | 692.59 | 692.22 | 695.16 | 695.14 |
| 75-46-7 | $CHF_3$ | C1s | 297.51 | 297.44 | 299.39 | 299.39 |
| 67-56-1 | $CH_3OH$ | O1s | 537.84 | 537.79 | 539.86 | 539.85 |
| 67-56-1 | $CH_3OH$ | C1s | 291.41 | 291.35 | 293.14 | 293.13 |
| 50-00-0 | $CH_2O$ | O1s | 538.14 | 538.20 | 540.49 | 540.46 |
| 50-00-0 | $CH_2O$ | C1s | 293.48 | 293.30 | 295.22 | 295.21 |
| 115-10-6 | $CH_3OCH_3$ | O1s | 537.40 | 537.45 | 539.42 | 539.40 |
| 115-10-6 | $CH_3OCH_3$ | C1s | 291.22 | 290.93 | 292.90 | 292.90 |
| 64-18-6 | HCOOH | O1s (OH) | 539.37 | 539.40 | 541.55 | 541.53 |
| 64-18-6 | HCOOH | O1s (C=O) | 537.47 | 537.64 | 539.80 | 539.79 |
| 64-18-6 | HCOOH | C1s | 294.34 | 294.39 | 296.09 | 296.10 |
| 67-64-1 | $(CH_3)_2CO$ | O1s | 536.56 | 536.66 | 538.77 | 538.76 |
| 67-64-1 | $(CH_3)_2CO$ | C1s (C=O) | 292.56 | 292.58 | 293.06 | 294.24 |
| 67-64-1 | $(CH_3)_2CO$ | C1s ($CH_3$) | 290.12 | 290.00 | 291.83 | 291.82 |
| 107-31-3 | $HCO_2CH_3$ | O1s ($OCH_3$) | 538.65 | 538.70 | 540.83 | 540.81 |
| 107-31-3 | $HCO_2CH_3$ | O1s (C=O) | 537.01 | 537.10 | 539.31 | 539.30 |
| 64-19-7 | $CH_3COOH$ | O1s (OH) | 538.79 | 538.75 | 540.89 | 540.87 |
| 64-19-7 | $CH_3COOH$ | O1s (C=O) | 536.78 | 537.26 | 539.01 | 539.00 |
| 64-19-7 | $CH_3COOH$ | C1s (COOH) | 293.97 | 293.97 | 295.61 | 295.61 |
| 64-19-7 | $CH_3COOH$ | C1s ($CH_3$) | 290.55 | 290.40 | 292.23 | 292.23 |
| 7732-18-5 | $H_2O$ | O1s | 538.59 | 538.58 | 540.67 | 540.66 |
| 10028-15-6 | $O_3$ | O1s middle | 543.25 | 545.68 | 548.05 | 548.00 |
| 10028-15-6 | $O_3$ | O1s terminal | 540.51 | 540.65 | 542.92 | 542.88 |
| 7782-44-7 | $O_2$ | O1s weaker | 541.98 | 542.15 | 544.48 | 544.46 |
| 7782-44-7 | $O_2$ | O1s stronger | 541.98 | 542.15 | 544.48 | 544.47 |
| 7727-37-9 | $N_2$ | N1s | 408.70 | 408.81 | 410.74 | 410.74 |
| 7664-41-7 | $NH_3$ | N1s | 404.63 | 404.43 | 406.33 | 406.26 |
| 74-90-8 | HCN | N1s | 405.75 | 405.75 | 407.76 | 407.77 |

**Table S2:** Continued

| name | formula | core level | CD | CD-WAC(20, 20, 200) | CD | CD-WAC(20, 20, 200) |
|---|---|---|---|---|---|---|
| | | | | | | |
| 74-90-8 | HCN | C1s | 292.50 | 292.57 | 294.13 | 294.11 |
| 75-05-8 | $CH_3CN$ | N1s | 404.49 | 404.46 | 406.48 | 406.46 |
| 75-05-8 | $CH_3CN$ | C1s ($CH_3$) | 291.66 | 291.63 | 293.39 | 293.38 |
| 75-05-8 | $CH_3CN$ | C1s (CN) | 291.69 | 291.70 | 293.31 | 293.30 |
| 56-40-6 | $C_2H_5NO_2$ | O1s (OH) | 538.79 | 538.79 | 540.88 | 540.87 |
| 56-40-6 | $C_2H_5NO_2$ | O1s (C=O) | 536.87 | 537.64 | 539.10 | 539.08 |
| 56-40-6 | $C_2H_5NO_2$ | N1s | 404.50 | 404.23 | 406.18 | 406.18 |
| 56-40-6 | $C_2H_5NO_2$ | C1s (COOH) | 293.71 | 293.67 | 295.39 | 295.37 |
| 56-40-6 | $C_2H_5NO_2$ | C1s ($CH_2$) | 291.12 | 291.13 | 292.84 | 292.84 |
| 110-86-1 | $C_5H_5N$ | N1s | 403.69 | 403.73 | 405.58 | 405.54 |
| 109-97-7 | $C_4H_4NH$ | N1s | 404.98 | 405.12 | 406.97 | 406.98 |
| 62-53-3 | $C_6H_5NH_2$ | N1s | 404.04 | 403.97 | 405.92 | 405.89 |
| 57-13-6 | $CO(NH_2)_2$ | O1s | 535.64 | 535.91 | 537.86 | 537.86 |
| 57-13-6 | $CO(NH_2)_2$ | N1s | 404.95 | 404.99 | 406.78 | 406.63 |
| 57-13-6 | $CO(NH_2)_2$ | C1s | 293.45 | 293.44 | 295.07 | 295.07 |
| 74-89-5 | $CH_3NH_2$ | N1s | 404.26 | 404.05 | 406.04 | 406.03 |
| 98-95-3 | $C_6H_5NO_2$ | O1s | 537.36 | 537.32 | 539.46 | 539.44 |
| 98-95-3 | $C_6H_5NO_2$ | N1s | 410.32 | 410.31 | 412.15 | 412.14 |
| 98-95-3 | $C_6H_5NO_2$ | C1s (C1) | 291.07 | 290.98 | 292.67 | 292.65 |
| 98-95-3 | $C_6H_5NO_2$ | C1s (C2-4) | 290.13 | 290.14 | 291.82 | 291.79 |
| 71-43-2 | $C_6H_6$ | C1s | 289.41 | 289.41 | 291.08 | 291.03 |
| 536-74-3 | $C_8H_6$ | C1s (C3) | 290.04 | 290.01 | 291.76 | 291.73 |
| 536-74-3 | $C_8H_6$ | C1s (C2) | 289.60 | 289.53 | 291.34 | 291.31 |
| 536-74-3 | $C_8H_6$ | C1s (C4-6) | 289.41 | 289.36 | 291.18 | 291.16 |
| 536-74-3 | $C_8H_6$ | C1s (C1) | 289.13 | 289.09 | 290.95 | 290.92 |
| MAE | | | | $1.476 \cdot 10^{-1}$ | | $3.681 \cdot 10^{-2}$ |
| MAD | | | | $4.891 \cdot 10^{-2}$ | | $6.450 \cdot 10^{-3}$ |

**Table S3:** Comparison of the CORE65 binding energies obtained with CD and CD-WAC at the $G_{\Delta H}W_0$@PBE level of theory with the cc–pvTZ basis set. The MAE and MAD values of CD-WAC with respect to CD are also reported.

| | | | $GW_{\Delta H}$@PBE | |
|---|---|---|---|---|
| name | formula | core level | CD | CD-WAC(20, 20, 200) |
| 74-82-8 | $CH_4$ | C1s | 290.00 | 290.00 |
| 74-84-0 | $C_2H_6$ | C1s | 289.89 | 289.89 |
| 74-85-1 | $C_2H_4$ | C1s | 290.10 | 290.10 |
| 74-86-2 | $C_2H_2$ | C1s | 290.50 | 290.44 |
| 630-08-0 | CO | O1s | 541.44 | 541.44 |
| 630-08-0 | CO | C1s | 295.15 | 295.15 |
| 124-38-9 | $CO_2$ | O1s | 540.15 | 540.15 |
| 124-38-9 | $CO_2$ | C1s | 296.26 | 296.26 |
| 75-73-0 | $CF_4$ | F1s | 693.61 | 693.61 |
| 75-73-0 | $CF_4$ | C1s | 300.16 | 300.15 |
| 593-53-3 | $CH_3F$ | F1s | 691.23 | 691.23 |
| 593-53-3 | $CH_3F$ | C1s | 292.57 | 292.57 |
| 75-46-7 | $CHF_3$ | F1s | 692.80 | 692.80 |
| 75-46-7 | $CHF_3$ | C1s | 297.69 | 297.69 |

**Table S3:** Continued

| name | formula | core level | CD | CD-WAC(20, 20, 200) |
|---|---|---|---|---|
| 67-56-1 | $CH_3OH$ | O1s | 537.96 | 537.96 |
| 67-56-1 | $CH_3OH$ | C1s | 291.53 | 291.53 |
| 50-00-0 | $CH_2O$ | O1s | 538.36 | 538.36 |
| 50-00-0 | $CH_2O$ | C1s | 293.60 | 293.60 |
| 115-10-6 | $CH_3OCH_3$ | O1s | 537.51 | 537.51 |
| 115-10-6 | $CH_3OCH_3$ | C1s | 291.32 | 291.32 |
| 64-18-6 | HCOOH | O1s (OH) | 539.47 | 539.47 |
| 64-18-6 | HCOOH | O1s (C=O) | 537.65 | 537.65 |
| 64-18-6 | HCOOH | C1s | 294.50 | 294.50 |
| 67-64-1 | $(CH_3)_2CO$ | O1s | 536.69 | 536.69 |
| 67-64-1 | $(CH_3)_2CO$ | C1s (C=O) | 292.55 | 292.63 |
| 67-64-1 | $(CH_3)_2CO$ | C1s ($CH_3$) | 290.27 | 290.27 |
| 107-31-3 | $HCO_2CH_3$ | O1s ($OCH_3$) | 538.79 | 538.79 |
| 107-31-3 | $HCO_2CH_3$ | O1s (C=O) | 537.19 | 537.19 |
| 64-19-7 | $CH_3COOH$ | O1s (OH) | 538.87 | 538.87 |
| 64-19-7 | $CH_3COOH$ | O1s (C=O) | 536.93 | 536.93 |
| 64-19-7 | $CH_3COOH$ | C1s (COOH) | 294.05 | 294.06 |
| 64-19-7 | $CH_3COOH$ | C1s ($CH_3$) | 290.65 | 290.65 |
| 7732-18-5 | $H_2O$ | O1s | 538.68 | 538.69 |
| 10028-15-6 | $O_3$ | O1s middle | 545.91 | 545.91 |
| 10028-15-6 | $O_3$ | O1s terminal | 540.63 | 540.63 |
| 7782-44-7 | $O_2$ | O1s weaker | 542.10 | 543.00 |
| 7782-44-7 | $O_2$ | O1s stronger | 542.10 | 542.10 |
| 7727-37-9 | $N_2$ | N1s | 408.89 | 408.89 |
| 7664-41-7 | $NH_3$ | N1s | 404.47 | 404.19 |
| 74-90-8 | HCN | N1s | 405.85 | 405.85 |
| 74-90-8 | HCN | C1s | 292.55 | 292.54 |
| 75-05-8 | $CH_3CN$ | N1s | 404.57 | 404.56 |
| 75-05-8 | $CH_3CN$ | C1s ($CH_3$) | 291.82 | 291.82 |
| 75-05-8 | $CH_3CN$ | C1s (CN) | 291.77 | 291.77 |
| 56-40-6 | $C_2H_5NO_2$ | O1s (OH) | 538.88 | 538.88 |
| 56-40-6 | $C_2H_5NO_2$ | O1s (C=O) | 537.00 | 537.00 |
| 56-40-6 | $C_2H_5NO_2$ | N1s | 404.62 | 404.44 |
| 56-40-6 | $C_2H_5NO_2$ | C1s (COOH) | 293.80 | 293.83 |
| 56-40-6 | $C_2H_5NO_2$ | C1s ($CH_2$) | 291.29 | 291.28 |
| 110-86-1 | $C_5H_5N$ | N1s | 403.89 | 403.85 |
| 109-97-7 | $C_4H_4NH$ | N1s | 404.85 | 405.21 |
| 62-53-3 | $C_6H_5NH_2$ | N1s | 404.30 | 404.19 |
| 57-13-6 | $CO(NH_2)_2$ | O1s | 535.77 | 535.77 |
| 57-13-6 | $CO(NH_2)_2$ | N1s | 405.02 | 405.04 |
| 57-13-6 | $CO(NH_2)_2$ | C1s | 293.61 | 293.55 |
| 74-89-5 | $CH_3NH_2$ | N1s | 404.35 | 404.35 |
| 98-95-3 | $C_6H_5NO_2$ | O1s | 537.34 | 537.34 |
| 98-95-3 | $C_6H_5NO_2$ | N1s | 410.36 | 410.38 |
| 98-95-3 | $C_6H_5NO_2$ | C1s (C1) | 291.16 | 291.17 |
| 98-95-3 | $C_6H_5NO_2$ | C1s (C2-4) | 290.23 | 290.22 |
| 71-43-2 | $C_6H_6$ | C1s | 289.49 | 289.48 |
| 536-74-3 | $C_8H_6$ | C1s (C3) | 290.18 | 290.20 |
| 536-74-3 | $C_8H_6$ | C1s (C2) | 289.71 | 289.73 |
| 536-74-3 | $C_8H_6$ | C1s (C4-6) | 289.54 | 289.54 |

**Table S3:** Continued

| name | formula | core level | CD | CD-WAC(20, 20, 200) |
|---|---|---|---|---|
| | | | | |
| 536-74-3 | $C_8H_6$ | C1s (C1) | 289.19 | 289.18 |
| MAE | | | | $2.625 \cdot 10^{-2}$ |
| MAD | | | | $4.000 \cdot 10^{-4}$ |

## 2 Padé interpolants and Thiele's reciprocal differences

One possible way of performing the analytic continuation of a complex function is obtaining its Padé approximant, which is a rational function of the form:

$$T(z) = \frac{P_L(z)}{Q_M(z)} \tag{1}$$

where $P_L$ and $Q_M$ are polynomials of degree $L$ and $M$ at most, respectively. It can be shown that the power series of the interpolant $T$ is equivalent to that of the interpolated function,[1] and this is the key motivation to use them in analytic continuation.

In the $GW$ bibliography, the analytic continuation is usually introduced using the following N–point interpolant:

$$T_N(z) = \frac{\sum_{i=0}^{\frac{N-1}{2}} p_i z^i}{1 + \sum_{i=1}^{\frac{N}{2}} q_i z^i} = \frac{A_N}{B_N} \tag{2}$$

A direct way of finding the $p_i$ and $q_i$ coefficients above is to solve the linear system of $2N$ equations generated from $N$ interpolation points.[2] In FHI-aims however, we use a simpler approach based on Thiele's reciprocal different algorithm:

$$T_N(z) = \cfrac{a_1}{1 + \cfrac{a_2(z-\omega_1)}{1 + \cfrac{a_3(z-\omega_2)}{\ddots \quad 1 + \cfrac{a_p(z-\omega_{p-1})}{1 + (z-\omega_p)g_{p+1}(z)}}}} \tag{3}$$

with the definition:

$$g_p(\omega_i) = \begin{cases} W(\omega_i) & p = 1 \\ \frac{g_{p-1}(\omega_{p-1}) - g_{p-1}(\omega_i)}{(\omega_i - \omega_{p-1}) g_{p-1}(\omega_i)} & p > 1 \end{cases} \tag{4}$$

and the properties:

$$\begin{aligned} T_N(\omega_i) &= W(\omega_i) \qquad i = 1, \ldots, N \\ a_i &= g_i(\omega_i) \qquad i = 1, \ldots, N \end{aligned} \tag{5}$$

In the above expressions we have employed as an example $N$ reference ordered pairs $(\omega_i, W(\omega_i))$ of frequencies and corresponding screened Coulomb interaction. This approach has the advantage of being efficiently computed by recursion and memoization.

It is possible to establish a correspondence[1] between the interpolant in the forms 2 and 3. Indeed, for the $N+1$ convergent we have:

$$\frac{A_{N+1}}{B_{N+1}} = \frac{A_N + (z-\omega_N)a_{N+1}A_{N-1}}{B_N + (z-\omega_N)a_{N+1}B_{N-1}} \tag{6}$$

with

$$A_{-1} = 0, \quad A_0 = a_0, \quad B_{-1} = 1, \quad B_0 = 1 \tag{7}$$

Many of the above results can be straightforwardly proved by induction. As an example, we include the proof of the second expression on Equation 5

*Proof.* $a_i = g_i(\omega_i) \quad i = 1, \ldots, N$

- Base case ($p = 1$)

The expression $a_1 = g_1(\omega_1)$ holds trivially from Equations 3 and 5:

$$T_N(\omega_1) = a_1 = W(\omega_1) = g_1(\omega_1) \tag{8}$$

- Inductive step ($p \to p + 1$)

Our hypothesis is that if $a_p = g_p(\omega_p)$, then $a_{p+1} = g_{p+1}(\omega_{p+1})$. We start with the definition of $g_{p+1}(z)$ for an arbitrary complex argument $z$ and index $p + 1 < N$:

$$g_{p+1}(z) = \frac{g_p(\omega_p) - g_p(z)}{(z - \omega_p)g_p(z)} \tag{9}$$

If we substitute $a_p$ in the above expression and then rearrange, we get:

$$g_p(z) = \frac{a_p}{1 + (z - \omega_p)g_{p+1}(z)} \tag{10}$$

By comparing the above expression with the general term in 3, we can see that the next reference point $\omega_{p+1}$ will be added as follows:

$$g_{p+1}(z) = \frac{a_{p+1}}{1 + (z - \omega_{p+1})g_{p+2}(z)} \tag{11}$$

Evaluating the former equation at $z = \omega_{p+1}$ we obtain $a_{p+1} = g_{p+1}(\omega_{p+1})$. □

## 3 Additional plots

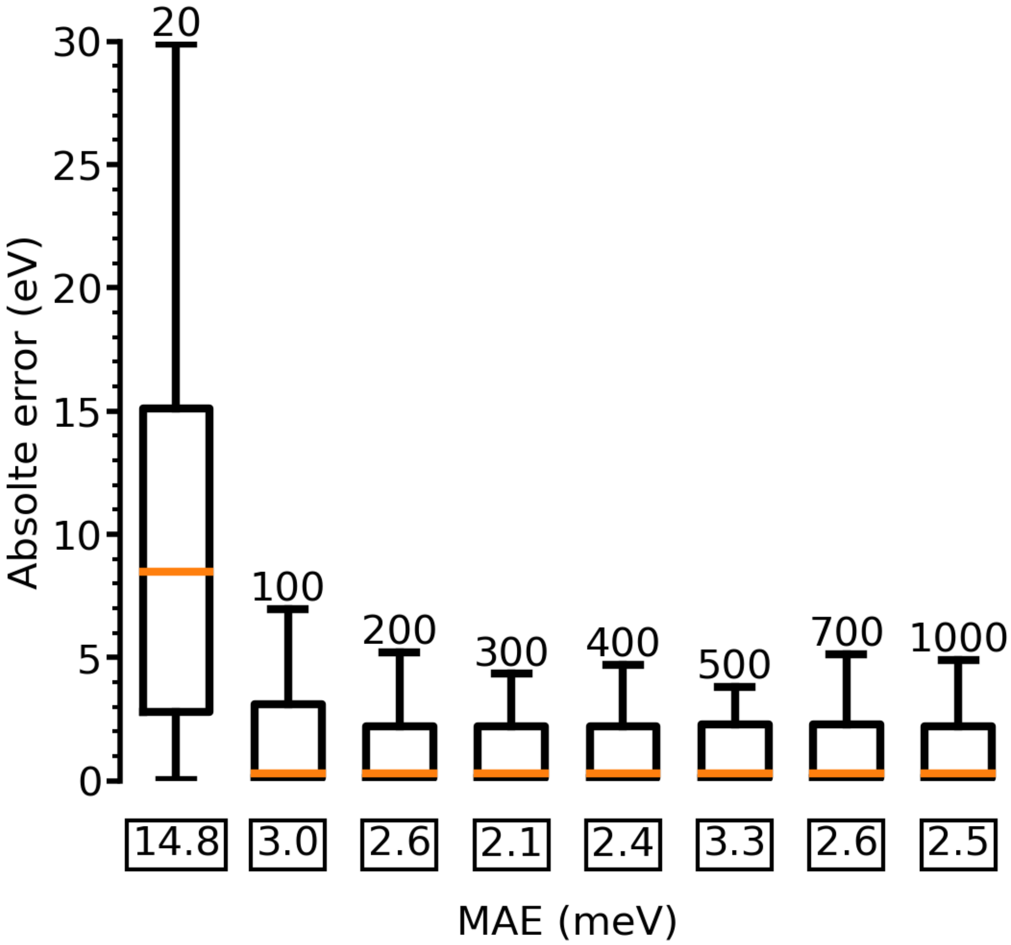


**Figure S1:** Box plots of the absolute errors of the CD-WAC(700,0,200) method with respect to CD for the CORE65 benchmark set at the $G_0W_0$@PBEh($\alpha$=0.45) level of theory and cc–pVTZ basis set. The numbers on top of the upper whiskers represent the corresponding value of the size of the $\omega_G$ grid. The corresponding MAEs are also reported. Boxes indicate the ”interquartile range” measuring where the bulk of the data are. The median is indicated by an orange line.

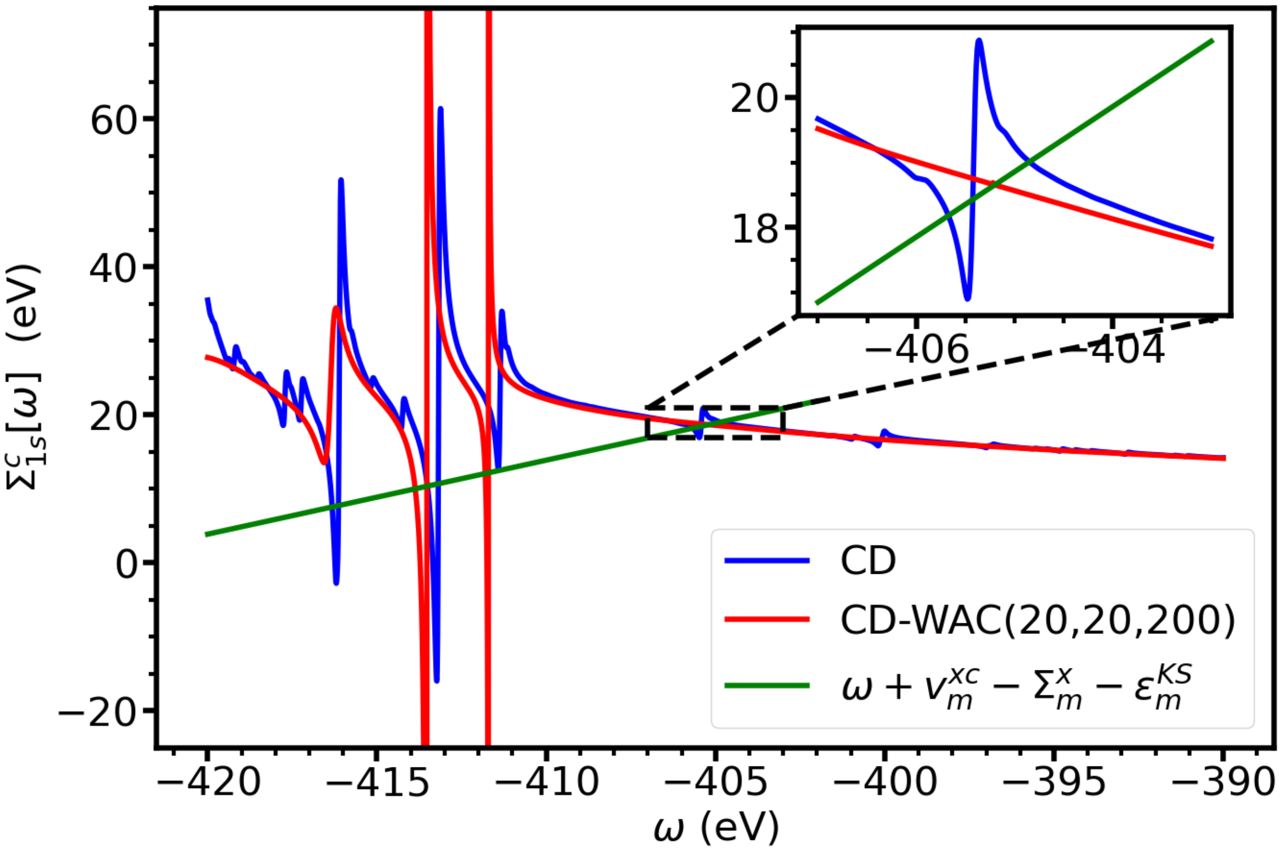


**Figure S2:** Self-energy matrix element for the N 1s core state of the pyrrole molecule (CAS 109-97-7). The plot showcases the comparison between CD and CD-WAC(20,20,200) at the $G_{\Delta H}W_0$@PBE level of theory and cc-pVTZ basis set. The interception with the green straight line gives the graphical solution to the quasiparticle equation.

## References


(1) George Jr, A.; others *Essentials of Padé approximants*; Elsevier, 1975.

(2) Beach, K.; Gooding, R.; Marsiglio, F. Reliable Padé analytical continuation method based on a high-accuracy symbolic computation algorithm. *Phys. Rev. B* **2000**, *61*, 5147.
